# Supplementary material for: Competing Gauge Fields and Entropically-Driven Spin Liquid to Spin Liquid Transition in non-Kramers Pyrochlores
Source: arXiv:2310.16682 source file (2024-09-03)
Supplement: Supplementary file 1 [file Supplementary_Material.pdf]

# Supplemental Material for "Competing Gauge Fields and Entropically-Driven Spin Liquid to Spin Liquid Transition in non-Kramers Pyrochlores"

Daniel Lozano-Gómez,[1,2,3] Vincent Noculak,[4,5] Jaan Oitmaa,[6] Rajiv R. P. Singh,[7] Yasir Iqbal,[8] Johannes Reuther,[4,5,8] and Michel J. P. Gingras[1]

[1]*Department of Physics and Astronomy, University of Waterloo, Waterloo, Ontario N2L 3G1, Canada*
[2]*Institut für Theoretische Physik and Würzburg-Dresden Cluster of Excellence ct.qmat*
[3]*Technische Universität Dresden, 01062 Dresden, Germany*
[4]*Dahlem Center for Complex Quantum Systems and Fachbereich Physik, Freie Universität Berlin, 14195 Berlin, Germany*
[5]*Helmholtz-Zentrum Berlin für Materialien und Energie, Hahn-Meitner-Platz 1, 14109 Berlin, Germany*
[6]*School of Physics, The University of New South Wales, Sydney 2052, Australia*
[7]*Department of Physics, University of California Davis, California 95616, USA*
[8]*Department of Physics and Quantum Centre of Excellence for Diamond and Emergent Materials (QuCenDiEM), Indian Institute of Technology Madras, Chennai 600036, India*

## CONTENTS

SI-1. DM Vectors 2

SI-2. Interaction Matrix Bands 2

SI-3. Structure Factors 3

SI-4. Irreducible Representations Parameters 3

SI-5. Irreducible Representations Basis 4

SI-6. Further Details on the SCGA 5

SI-7. Long-wavelength Theory 6

SI-8. Iterative Minimization 7

SI-9. Classical Low-Temperature Expansion 8

SI-10. Monte Carlo Temperature Phase Diagram for the Heisenberg and DM Model 9

SI-11. Monte Carlo Temperature-Dependence Spin Structure Factors 9

SI-12. Neutron Structure Factor of the DQQ Model 10

SI-13. Dual DQQ Model (DQQ*) Spin Structure Factors 12

SI-14. Pseudo-Fermion Functional Renormalization Group (PFFRG) Method 13

SI-15. PFFRG Spin Structure Factors in the Vicinity of the DQQ Point 14

SI-16. High-Temperature Series Expansion (HTSE) 14

References 16

## SI-1. DM VECTORS

Here, we list the Dzyaloshinskii-Moriya (DM) vectors $\boldsymbol{d}_{ij}$ used in the Hamiltonian of (4) in the main text. These vectors can be obtained by following the Moriya rules [1–3], resulting in six DM vectors corresponding to the six bonds found in a tetrahedron, namely,

$$\boldsymbol{d}_{01} = (-1, 1, 0), \quad \boldsymbol{d}_{02} = (1, 0, -1), \quad \boldsymbol{d}_{03} = (0, -1, 1), \tag{S1}$$

$$\boldsymbol{d}_{12} = (0, 1, 1), \quad \boldsymbol{d}_{13} = (-1, 0, -1), \quad \boldsymbol{d}_{23} = (1, 1, 0). \tag{S2}$$

Here, the subscripts $ij$ index the four sublattices $(0, 1, 2, 3)$ of the primitive tetrahedral cell. The face-centered cubic (FCC) primitive lattice translation vectors are:

$$\boldsymbol{r}_0 = \Big(0,0,0\Big), \quad \boldsymbol{r}_1 = \frac{a}{4}\Big(1,1,0\Big), \quad \boldsymbol{r}_2 = \frac{a}{4}\Big(1,0,1\Big), \quad \boldsymbol{r}_3 = \frac{a}{4}\Big(0,1,1\Big), \tag{S3}$$

where $a$ is the length of a conventional cubic unit cell. From here on, we take $a = 1$.

## SI-2. INTERACTION MATRIX BANDS

In this section, we give the eigenvalues of the interaction matrix $\boldsymbol{M}_{ij}$ in (2) in the main text (with $J = 1$ and $D = -2J$) in reciprocal space and along high-symmetry paths in the $[hh\ell]$ and $[hk0]$ planes, see Fig. SI-2.1. We find that the lowest four bands are completely flat and degenerate, hinting at the extensive degeneracy of the ground state manifold. It is also worth noting that, out of the four flat bands, two of these correspond to the local-$z$ degrees of freedom whereas the other two to the local-$xy$ degrees. The separation and identification of these bands with those degrees of freedom are obtained by considering the interaction matrix in reciprocal space, $\boldsymbol{M}(\boldsymbol{q})$, as a sum of two interaction matrices: one constructed by only considering the interactions between only local-$z$ degrees of freedom and another with only the local-$xy$. In other words, considering the local-$z$ interaction matrix uniquely composed by the $J_{zz}$ term of (2), while the local-$xy$ interaction matrix is composed by the remaining $J_{\pm}$ and $J_{\pm\pm}$ terms.

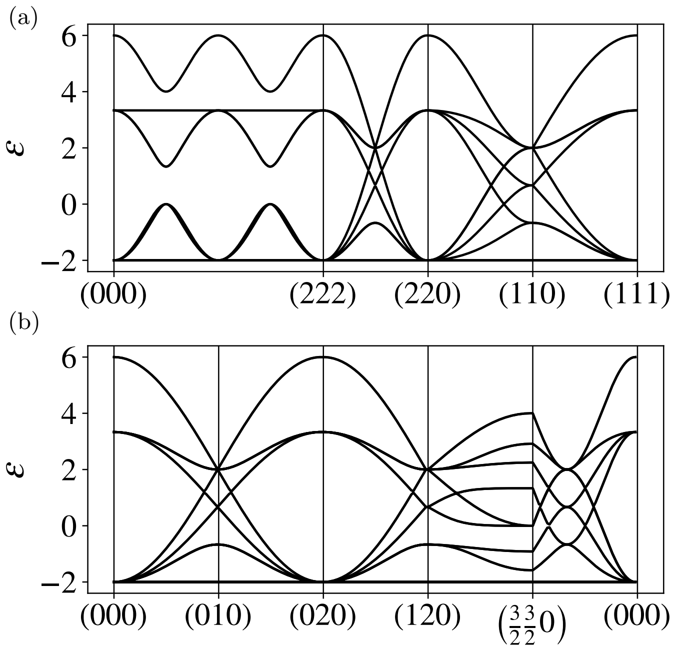


FIG. SI-2.1: Energy bands of the interaction matrix of the Heisenberg and DM model with $D/J = -2$ in units of $J$ plotted, along high-symmetry paths in the $[hh\ell]$ and $[hk0]$ planes illustrated in panels (a) and (b), respectively.

## SI-3. STRUCTURE FACTORS

In order to study the correlations between the spins in the system, we study the unpolarized energy-integrated neutron structure factor

$$\mathcal{S}_\perp(\boldsymbol{q}) = \sum_{\alpha\beta}\sum_{\mu\nu}\left(\delta_{\alpha\beta} - \frac{q^\alpha q^\beta}{q^2}\right)\langle \mu_a^\alpha(-\boldsymbol{q})\mu_b^\beta(\boldsymbol{q})\rangle, \tag{S1}$$

as well as the non-spin-flip (NSF) and spin-flip (SF) structure factors

$$\mathcal{S}_\perp^{\rm NSF}(\boldsymbol{q}) = \sum_{\alpha\beta}\sum_{\mu\nu} z_s^\alpha z_s^\beta \langle \mu_a^\alpha(-\boldsymbol{q})\mu_b^\beta(\boldsymbol{q})\rangle, \tag{S2}$$

$$\mathcal{S}_\perp^{\rm SF}(\boldsymbol{q}) = \mathcal{S}_\perp(\boldsymbol{q}) - \mathcal{S}_\perp^{\rm NSF}(\boldsymbol{q}), \tag{S3}$$

where the greek letters, $\{\alpha,\beta\}$, label the magnetic moment components, the roman letters $\{a,b\}$ the sublattice coordinates, $\boldsymbol{z}_s$ corresponds to the polarization direction of the incident neutron [4], and $\boldsymbol{\mu}_a(\boldsymbol{q})$ is the Fourier transform of the magnetic moment $\boldsymbol{\mu}_{ia}$, defined as $\boldsymbol{\mu}_a(\boldsymbol{q}) = \frac{1}{\sqrt{N}}\sum_i \boldsymbol{\mu}_{ia} e^{-i((\boldsymbol{R}_i+\boldsymbol{r}_a)\cdot\boldsymbol{q})}$, where $\boldsymbol{R}_i$ labels the FCC primitive translation lattice vectors. Here, $\boldsymbol{z}_s$ is perpendicular to the scattering plane measured. In terms of the spin degrees of freedom, $\boldsymbol{S}_{ia}$, the magnetic moments are defined as

$$\mu_{ia}^\alpha = \sum_\beta g_a^{\alpha,\beta} S_{ia}^\beta, \tag{S4}$$

where $g_a^{\alpha,\beta}$ is the magnetic $g$-tensor which in the local basis takes the simplified form

$$g = \begin{pmatrix} g^\perp & 0 & 0 \\ 0 & g^\perp & 0 \\ 0 & 0 & g^{zz} \end{pmatrix}. \tag{S5}$$

From here on, we refer to (S1)-(S3) as the "neutron structure factors" whenever we use the non-Kramers $g$-tensor (i.e. $g^{zz}=1$ and $g^\perp = 0$), and to "spin structure factors" whenever we use an isotropic $g$-tensor (i.e. $g^{zz}=1$ and $g^\perp=1$). In particular in Figures 1, 2 and 5 of the main text, we consider the spin structure factor. This choice is made therein in order to expose the key and prominent anisotropic features of the correlation function between the local-$z$ and local-$xy$ components of the spins $\boldsymbol{S}_{ia}$. To compute the physically meaningful and experimentally measurable neutron structure factor discussed in Sections SI-12 we must use an anisotropic $g$-tensor which only retains the dipolar local-$z$ component of every spin while ignoring the electric quadrupole degrees of freedom which are represented by the $xy$ components of $\boldsymbol{S}_{ia}$ [5, 6].

## SI-4. IRREDUCIBLE REPRESENTATIONS PARAMETERS

As discussed in the main text, the irreducible representation energy eigenvalues $\{a_I\}$ for the general bilinear nearest-neighbour Hamiltonian model of (2) in the main text are linear functions of the $\{J_{zz}, J_\pm, J_{\pm\pm}, J_{z\pm}\}$ spin-spin couplings [7], namely

$$a_{A_2} = 3J_{zz}, \tag{S1}$$

$$a_E = -6J_\pm, \tag{S2}$$

$$a_{T_2} = 2J_\pm - 4J_{\pm\pm}, \tag{S3}$$

$$a_{T_1^{\rm Ice}} = -J_{zz}, \tag{S4}$$

$$a_{T_1^{xy}} = 2J_\pm + 4J_{\pm\pm}, \tag{S5}$$

$$a_{T_1^{\rm mix}} = -8J_{z\pm}. \tag{S6}$$

where the $a_{T_1^{\rm mix}}$ parameter corresponds to a mixing between the two $T_1$ irreps which can be eliminated by a basis rotation [7, 8]. For non-Kramers ions, where the local transverse components are quadrupolar, such as for our DQQ

model with $D/J = -2$, the mixing term $a_{T_1^{\rm mix}}$ vanishes because $J_{z\pm} = 0$ [5, 9]. Using the relation between the local interaction parameters and the Heisenberg and DM coupling, namely $\{J_{zz}, J_{\pm}, J_{\pm\pm}, J_{z\pm}\} = \{-\frac{1}{3}(-J+4D), \frac{1}{6}(-J-2D), \frac{1}{3}(-J+D), \frac{1}{3\sqrt{2}}(-2J-D)\}$ from Ref.[8], we obtain the following values for the $a_I$ parameters for the DQQ model ($D/J = -2$)

$$a_{A_2} = 9J, \tag{S7}$$
$$a_E = -3J, \tag{S8}$$
$$a_{T_2} = 5J, \tag{S9}$$
$$a_{T_1^{\rm Ice}} = -3J, \tag{S10}$$
$$a_{T_1^{xy}} = -3J. \tag{S11}$$

## SI-5. IRREDUCIBLE REPRESENTATIONS BASIS

An irrep decomposition of the Hamiltonian $\mathcal{H}^{\boxtimes}$ can be understood as a spectral decomposition where the resulting eigenvectors (irreps) span non-overlapping subspaces under the action of the tetrahedral group $T_d$. In this language, irreps correspond to the spin configurations which are eigenvectors of the single tetrahedron Hamiltonian $\mathcal{H}^{\boxtimes}$. The spin configurations corresponding to the different irreps can be constructed using the *local* basis directions of the spins. For the $0^{\rm th}$ sublattice the local spin directions, $\boldsymbol{x}_0$, $\boldsymbol{y}_0$ and $\boldsymbol{z}_0$, are given in the global Cartesian coordinate frame by

$$\boldsymbol{x}_0 = \frac{1}{\sqrt{6}}\begin{pmatrix}-1\\-1\\2\end{pmatrix}, \quad \boldsymbol{y}_0 = \frac{1}{\sqrt{2}}\begin{pmatrix}1\\-1\\0\end{pmatrix}, \quad \boldsymbol{z}_0 = \frac{1}{\sqrt{3}}\begin{pmatrix}1\\1\\1\end{pmatrix},$$

where the local basis for the other sublattices can be obtained by application of other $T_d$ symmetry operations, see Fig. SI-5.1.

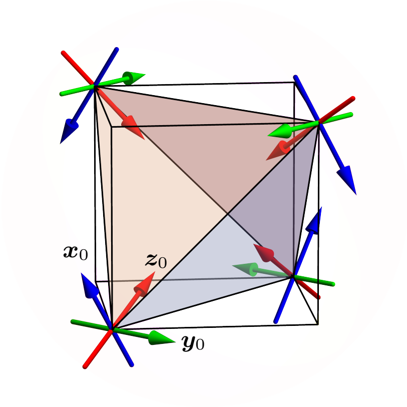


FIG. SI-5.1: Local sublattice basis where the blue directions correspond to the local $x$ direction, the green to the local $y$, and the red to the local $z$.

Using the local sublattice directions, the irrep modes in the global frame are discussed in Ref. [7] and defined as

$$m^{\boxtimes}_{A_2} = \frac{1}{2\sqrt{3}} \sum_a (\boldsymbol{z}_a \cdot \boldsymbol{S}_a), \tag{S1}$$

$$\boldsymbol{m}^{\boxtimes}_{E} = \frac{1}{2} \sum_a \begin{pmatrix} \frac{1}{\sqrt{6}} \boldsymbol{x}_a \cdot \boldsymbol{S}_a \\ \frac{1}{\sqrt{2}} \boldsymbol{y}_a \cdot \boldsymbol{S}_a \end{pmatrix}, \tag{S2}$$

$$\boldsymbol{m}^{\boxtimes}_{T_1^{xy}} = \frac{1}{\sqrt{96}} \sum_a \begin{pmatrix} 2\boldsymbol{x}_a \cdot \boldsymbol{S}_a (-1)^{\delta_{a,(2,3)}} \\ (-\boldsymbol{x}_a \cdot \boldsymbol{S}_\mu)\,(-1)^{\delta_{a,(1,3)}} \\ (-\boldsymbol{x}_a \cdot \boldsymbol{S}_\mu)(-1)^{\delta_{a,(1,2)}} \end{pmatrix} + \frac{3}{\sqrt{96}} \sum_a \begin{pmatrix} 0 \\ (\boldsymbol{y}_a \cdot \boldsymbol{S}_a)(-1)^{\delta_{a,(1,3)}} \\ (-\boldsymbol{y}_a \cdot \boldsymbol{S}_a)(-1)^{\delta_{a,(1,2)}} \end{pmatrix}, \tag{S3}$$

$$\boldsymbol{m}^{\boxtimes}_{T_1^{\mathrm{Ice}}} = \frac{1}{\sqrt{2}} \sum_a \begin{pmatrix} z_a^x z_a^z (\boldsymbol{z}_a \cdot \boldsymbol{S}_a) \\ z_a^y z_a^z (\boldsymbol{z}_a \cdot \boldsymbol{S}_a) \\ z_a^z z_a^z (\boldsymbol{z}_a \cdot \boldsymbol{S}_a) \end{pmatrix}, \tag{S4}$$

$$\boldsymbol{m}^{\boxtimes}_{T_2} = \frac{1}{2\sqrt{2}} \sum_a \begin{pmatrix} (\boldsymbol{z}_a \times \boldsymbol{S}_a)^x \\ (\boldsymbol{z}_a \times \boldsymbol{S}_a)^y \\ (\boldsymbol{z}_a \times \boldsymbol{S}_a)^z \end{pmatrix}, \tag{S5}$$

where $z_a^\alpha$ ($S_a^\alpha$) is the $\alpha$ component of the local-$z$ direction (spin $\boldsymbol{S}$) on sublattice $a$ expressed in the global Cartesian frame, and $\delta_{a,(b,c)}$ is a Kronecker delta which vanishes if $a \neq b$ or $a \neq c$. An example of the spin configurations for the various irreps is shown in Fig. SI-5.2. Finally, we define the irrep projection in a single tetrahedron as the magnitude of the irrep modes $|\boldsymbol{m}_I^{\boxtimes}|$ obtained from a spin configuration in a single tetrahedron. The probability distribution of the irrep projections for spin configurations on the full pyrochlore lattice is of special relevance in a spin liquid phase as it exposes the thermal population of each one of the irrep modes. These projections are shown in Fig. 3 in the main text for all the up tetrahedra, labeled $\hat{\boxtimes}$, with spin configurations sampled via classical Monte Carlo at different temperatures and in the physically pertinent regimes of the model (4) in the main text with $D/J = -2$.

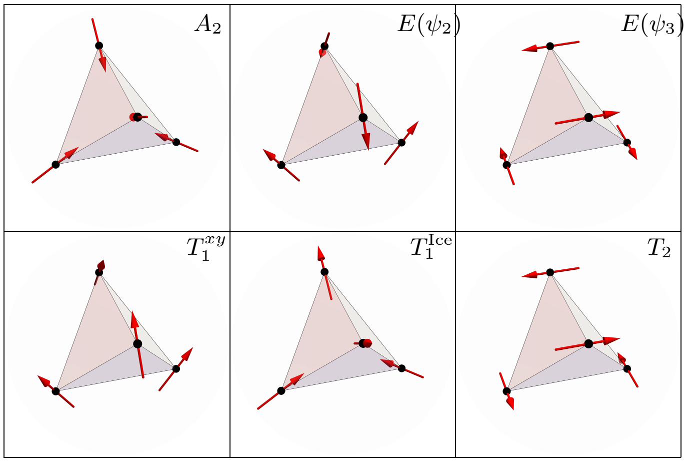


FIG. SI-5.2: Irreducible representation spin configurations on a single tetrahedron. Within these configurations, the $T_1^{\mathrm{Ice}}$ and the $T_1^{xy}$ modes correspond to splayed ferromagnetic configurations while all remaining modes are antiferromagnetic.

## SI-6. FURTHER DETAILS ON THE SCGA

For a general spin Hamiltonian with bilinear interactions

$$\mathcal{H} = \frac{1}{2} \sum_{i,j} \boldsymbol{S}_i \, \boldsymbol{M}_{ij} \, \boldsymbol{S}_j = \frac{1}{2} \sum_{ia,jb} \sum_{\alpha,\gamma} S_{ia}^\alpha \, \boldsymbol{M}_{ia,jb}^{\alpha,\gamma} \, S_{jb}^\gamma, \tag{S1}$$

where the sub-indices $i$ and $j$ label the primitive FCC vectors $\boldsymbol{R}_i$, and the additional indices in the interaction matrix $\boldsymbol{M}^{\alpha,\gamma}_{ia,jb}$ which we now write to explicitly express the sublattice and spin component structure resulting on a $\boldsymbol{q}$-dependent $12 \times 12$ matrix in reciprocal space, namely $\boldsymbol{M}^{\alpha\gamma}_{ab}(\boldsymbol{q})$. The spin-spin correlation function [4, 10] is given by the equation

$$\chi^{\alpha\gamma}_{ab} = \langle S^{\alpha}_{a}(\boldsymbol{q}) S^{\gamma}_{b}(-\boldsymbol{q})\rangle = \sum_{\boldsymbol{q}} (\beta \boldsymbol{M}^{\alpha\gamma}_{ab}(\boldsymbol{q}) + \lambda)^{-1}. \tag{S2}$$

For more details on the SCGA approximation, we refer the reader to Refs. [10, 11]. The SCGA applied to the DQQ model, for which we take $S = 1$, reveals how the Lagrange multiplier $\lambda$ plateaus to $\lambda_0 = 1$ at low temperatures, see Fig. SI-6.1. This value reflects the fraction of degenerate low-energy flat bands to the total number of bands in the interaction matrix which asymptotically approaches the value $\lambda_0 = 3(N_{\text{flat}}/12)$, where $N_{\text{flat}}$ are the number of flat bands ($N_{\text{flat}} = 4$, see Section SI-2 above) [12]. Using the values identified for $\lambda$, we compute the spin structure factor [4, 10, 11] (i.e., assuming an isotropic $g$-tensor as described in Section SI-3 to be

$$\mathcal{S}_{\perp}(\boldsymbol{q}) = \sum_{\alpha,\gamma} \sum_{\boldsymbol{q}} \left( \delta^{\alpha\gamma} - \frac{q^{\alpha} q^{\gamma}}{|\boldsymbol{q}|^2} \right) (\beta \boldsymbol{M}^{\alpha\gamma}_{ab}(\boldsymbol{q}) + \lambda)^{-1}. \tag{S3}$$

The spin structure factor in the $[hh\ell]$ and $[hk0]$ scattering planes is shown in Fig. 2 of the main text for various temperatures.

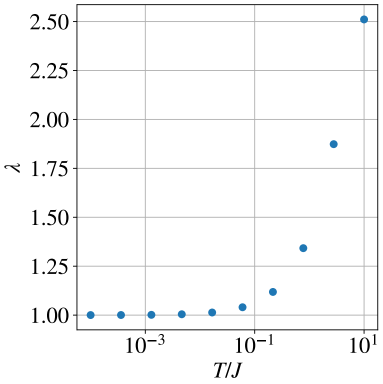


FIG. SI-6.1: Lagrange multiplier $\lambda$ computed from the SCGA for the DQQ model.

## SI-7. LONG-WAVELENGTH THEORY

The long-wavelength theory described in (7) of the main text is derived by first rewriting the Hamiltonian in (4) in terms of the irrep eigenvectors $\{\boldsymbol{m}_I\}$, as defined in Section SI-5 above, and then taking the small $\boldsymbol{q}$ limit, i.e. $|\boldsymbol{q}| \ll 1$. The Hamiltonian in terms of the irreps is obtained by defining a spin-to-irrep transformation $\mathbb{T}$, such that

$$\boldsymbol{m}^{\boxtimes} = \mathbb{T} \boldsymbol{S}^{\boxtimes},$$

where $\boldsymbol{m}^{\boxtimes}$ and $\boldsymbol{S}^{\boxtimes}$ are 12-dimensional vectors defined in a single tetrahedron. Given that the DQQ model corresponds to a non-Kramers model (since $J_{z\pm} = 0$ for $D/J = -2$) [5, 9], the resulting Hamiltonian becomes block-diagonal separating the local-$z$ irreps (the $A_2$ and the $T_1^{\text{Ice}}$ irreps) and the local-$xy$ irreps (the $E$ and the $T_1^{xy}$, and the $T_2$ irreps). In other words, we get

$$\mathcal{H} = \int d\boldsymbol{q}\, \boldsymbol{m}^{\boxtimes}(-\boldsymbol{q})^T \begin{pmatrix} (T_1^{\text{Ice}}, T_1^{\text{Ice}}) & (T_1^{\text{Ice}}, A_2) & 0 & 0 & 0 \\ (T_1^{\text{Ice}}, A_2) & (A_2, A_2) & 0 & 0 & 0 \\ 0 & 0 & (E, E) & (E, T_1^{xy}) & (E, T_2) \\ 0 & 0 & (E, T_1^{xy}) & (T_1^{xy}, T_1^{xy}) & (T_1^{xy}, T_2) \\ 0 & 0 & (E, T_2) & (T_1^{xy}, T_2) & (T_2, T_2) \end{pmatrix} \boldsymbol{m}^{\boxtimes}(-\boldsymbol{q}). \tag{S1}$$

Here the labels $(I_k, I_l)$ in the above $5 \times 5$ array corresponds to the $\boldsymbol{q}$-dependent bilinear interaction terms between the irreps $I_k$ and $I_l$ obtained from Fourier transforming the interaction matrix $\boldsymbol{M}_{ij}$. For better readability, here and in the main text, we have omitted the prefactor $(L/2\pi)^3$ from the momentum space integration measure which just leads to an overall rescaling of the theory. To obtain the low-temperature effective theory, we neglect the contribution of the high-energy $A_2$ and the $T_2$ irrep modes as these become depopulated in the low-temperature regime, see Fig. 3 and the accompanying discussion in the main text. In terms of (S1), neglecting such terms is equivalent to setting to 0 the blocks containing any the high-energy $A_2$ and the $T_2$ irreps, thus yielding the reduced effective low-energy Hamiltonian

$$\mathcal{H}_{=} \int d\boldsymbol{q}\; \widetilde{\boldsymbol{m}}^{\boxtimes}(-\boldsymbol{q})^T \begin{pmatrix} (T_1^{\text{Ice}}, T_1^{\text{Ice}}) & 0 & 0 \\ 0 & (E, E) & (E, T_1^{xy}) \\ 0 & (E, T_1^{xy}) & (T_1^{xy}, T_1^{xy}) \end{pmatrix} \widetilde{\boldsymbol{m}}^{\boxtimes}(-\boldsymbol{q}), \tag{S2}$$

where $\widetilde{\boldsymbol{m}}^{\boxtimes}$ is solely composed by the $E$, $T_1^{xy}$ and $T_1^{\text{Ice}}$ irreps. Employing the definitions in (5) and (6) in the main text, we may rewrite the effective Hamiltonian (S2) above to obtain the Hamiltonian in (7) in the main text composed of two terms: one $\boldsymbol{q}-$independent and another $\boldsymbol{q}-$dependent terms where we only consider terms up to quadratic order in $\boldsymbol{q}$. The $\boldsymbol{q}-$independent term corresponds to the ground-state energy

$$E_0 = -3J \int d\boldsymbol{q}\; \left\{ |\boldsymbol{B}^{\text{Ice}}|^2 + \text{Tr}\left[ (\mathcal{M}^{xy})^T \mathcal{M}^{xy} \right] \right\}, \tag{S3}$$

where

$$|\boldsymbol{B}^{\text{Ice}}|^2 + \text{Tr}\left[ (\mathcal{M}^{xy})^T \mathcal{M}^{xy} \right] = |\boldsymbol{m}_{T_1^{\text{Ice}}}|^2 + |\boldsymbol{m}_E|^2 + |\boldsymbol{m}_{T_1^{xy}}|^2. \tag{S4}$$

On the other hand, the $\boldsymbol{q}-$dependent term corresponds to the second term in (7) yielding the constraints in the fields $\boldsymbol{B}^{\text{Ice}}$ and $\mathcal{M}^{xy}$. The last term proportional to $\lambda$ in the SCGA long-wavelength theory in (7) is the Lagrange multiplier introduced to fix the spin-length constraint [10, 11], which in terms of the irreps yields a term

$$\lambda \sum_I |\boldsymbol{m}_I|^2. \tag{S5}$$

Using (S4) above, this last term can then be rewritten in terms of the fields in (5) and (6) yielding the last term in (7) (these latter three equations from the main text).

## SI-8. ITERATIVE MINIMIZATION

The iterative minimization (IM) scheme is a numerical technique to identify spin configurations that minimize the energy of a system given by a Hamiltonian

$$\mathcal{H} = -\frac{1}{2} \sum_i \boldsymbol{h}_i \cdot \boldsymbol{S}_i, \tag{S1}$$

where $\boldsymbol{h}_i$ is the molecular field at site $i$. Starting from the Hamiltonian in (4) in the main text, the procedure followed in this numerical approach is as follows: first, a random spin configuration is constructed. Then, at a randomly chosen site $i$, the molecular field $\boldsymbol{h}_i$, defined as

$$\boldsymbol{h}_i = \sum_{j@i} \left[ J\boldsymbol{S}_j - D(\boldsymbol{S}_j \times \boldsymbol{d}_{ij}) \right], \tag{S2}$$

where $j@i$ denotes $j$ nearest-neighbour of $i$, is calculated. The spin at site $i$ is then oriented along $\boldsymbol{h}_i$ effectively lowering the energy of the system. The spin reorientation is carried until the energy between subsequent updates is less than a threshold $\Delta E_{\text{cut}}$.

We applied IM onto the DQQ model to obtain the configurations used in the classical low-temperature expansion (CLTE) where we considered $\Delta E_{\text{cut}} = 10^{-11} J$ per spin. With the configurations sampled through IM, we computed

the spin structure factor and the irrep projection, see Fig. SI-8.1. The spin structure factors obtained from these configurations resemble those found by MC at temperatures just above $T^*$, see Fig. 1(c), (d) in the main text. On the other hand, the irrep projection of these configurations results in distributions where the $T_1^{\rm Ice}$, the $T_1^{xy}$, and the $E$ irreps have a roughly similar distribution ranging from 0 to 1, whereas the remaining high-energy $A_2$ and $T_2$ irreps have essentially vanishing distributions where the largest irrep projection was found to be at most $\sim 10^{-6}$.

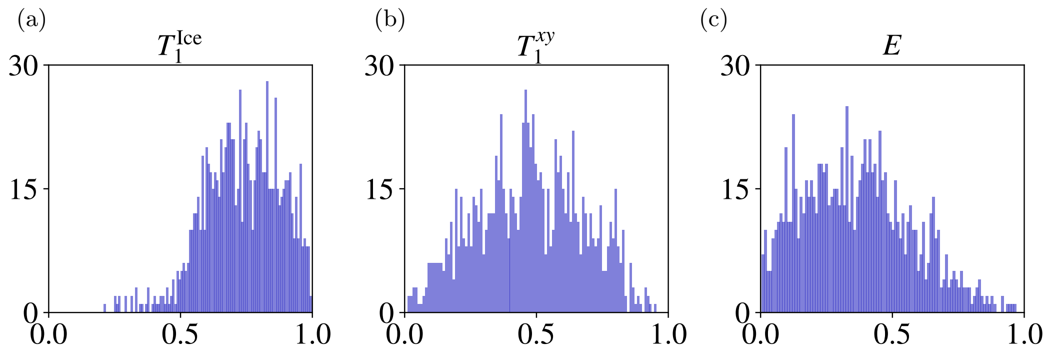


FIG. SI-8.1: Distribution of the irrep mode magnitude of all the *up* tetrahedra $\{|m_I^{\boxtimes}|\}$ of an iterative minimization (IM) sampled configuration of system size $L = 10$, for the $T_1^{\rm Ice}$ (a), for the $T_1^{xy}$ (b), and for the $E$ (c) irreps.

These IM results show that an unequal mixing between the $T_1^{\rm Ice}$, $T_1^{xy}$ and $E$ irreps on different tetrahedra is possible within a state of the ground state manifold (such as obtained by IM). For example, one possible ground state to achieve such mixed configuration is realized by parameterizing the spins on a tetrahedron in the following way

$$\begin{aligned} \boldsymbol{S}_0 &= (\cos(\beta), 0, \sin(\beta)), \\ \boldsymbol{S}_1 &= (\cos(\beta), 0, -\sin(\beta)), \\ \boldsymbol{S}_2 &= (\cos(\alpha), 0, \sin(\alpha)), \\ \boldsymbol{S}_3 &= (\cos(\alpha), 0, -\sin(\alpha)), \end{aligned} \tag{S3}$$

with the spins being expressed in the local coordinate system and $\alpha, \beta \in [0, 2\pi]$ being angles, which allows for a continuous degree of freedom along lines consisting of either sublattices 0 and 1, or 2 and 3. Figure SI-8.2 illustrates two instances of this parametrization for a set of connected tetrahedra. The continuous 1d degree of freedom consists of varying $\beta$ arbitrarily for the line of red spins. Note that in the state (S3), $\alpha$ and $\beta$ can be tuned to obtain a pure $E$ ($\psi_2$ for $\alpha = \beta = 0$ ), $T_1^{xy}$ ($\alpha = 0$ and $\beta = \pi$) or $T_1^{\rm Ice}$ ($\alpha = \beta = \frac{\pi}{2}$) state.

## SI-9. CLASSICAL LOW-TEMPERATURE EXPANSION

In this section, we elucidate the application of a classical low-temperature expansion on the pyrochlore lattice and show how a quadratic Hamiltonian describing the fluctuations about a low-temperature state is obtained. As stated in the Method section in the main text, we express the unit vector $\boldsymbol{S}_{ia}$ in (S1) above in the form given in (11) of the main text. This results in the following terms

$$\mathcal{H} = \mathcal{H}^{(0)} + \mathcal{H}^{(2)} + O(\delta n^3), \tag{S1}$$

where the zero-order term is the classical ground state energy of the configuration,

$$\mathcal{H}^{(0)} = \frac{S^2}{2} \sum_{ia,jb} \boldsymbol{M}^{\tilde{z}\tilde{z}}_{ia,jb}. \tag{S2}$$

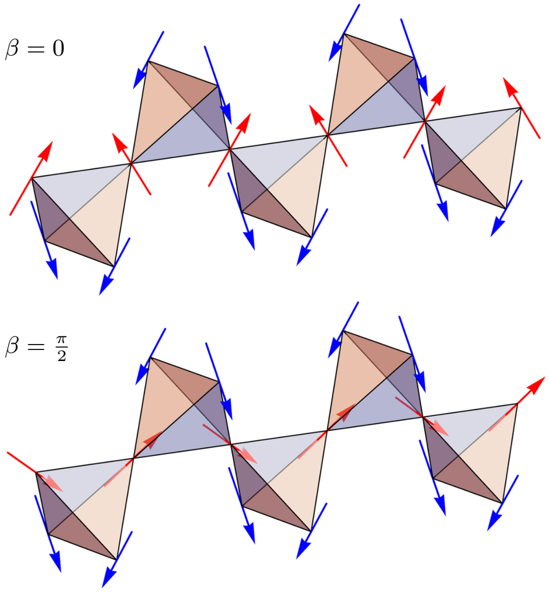


FIG. SI-8.2: The ground state spin configuration given by (S3) is shown for $\beta = 0$ and $\beta = \frac{\pi}{2}$ with $\alpha$ staying constant at $\alpha = 0$. Spins on sublattices 0 and 1 (2 and 3) are shown in blue (red).

Here, $\boldsymbol{M}^{\tilde{z}\tilde{z}}_{ia,jb}$ is the unitary-rotated $\boldsymbol{M}^{\alpha\beta}_{ia,jb}$ matrix along the low-temperature spin configurations at site $ia$ and $jb$ [7], and the second-order term is an effective quadratic Hamiltonian for the fluctuating components of the spins

$$\mathcal{H}^{(2)} = \frac{1}{2} \sum_{ia,jb} \sum_{\alpha,\gamma} \left( \delta n^{\alpha}_{ia} \boldsymbol{M}^{\alpha\gamma}_{ia,jb} \delta n^{\gamma}_{jb} - \delta_{\alpha\gamma} \delta n^{\alpha}_{ia} \boldsymbol{M}^{\tilde{z}\tilde{z}}_{ia,jb} \delta n^{\gamma}_{ia} \right). \tag{S3}$$

In practice, this procedure is equivalent to finding the Hessian matrix whose eigenvalues correspond to the energies of the quadratic modes, see Refs. [8, 13] for more details. This procedure is applied and discussed in the main text where the numerically obtained eigenvalue spectra for the states considered are shown in Fig. 4(a) and (b). We note that the numerically obtained eigenvalues below an approximate cutoff value of $J \times 10^{-9}$ fall below machine precision error when diagonalizing the quadratic Hamiltonian $\mathcal{H}^{(2)}$ and are therefore identified with zero-modes in the quadratic theory.

## SI-10. MONTE CARLO TEMPERATURE PHASE DIAGRAM FOR THE HEISENBERG AND DM MODEL

Here, in Fig. SI-10.1, we report the classical phase diagram of the Heisenberg and DM Hamiltonian parametrized as $\{J(\theta), D(\theta)\} = \{\cos\theta, \sin\theta\}$ where no order is found down to temperature $T \sim 10^{-4}$ in units of $J$ for the ratio $D/J = -2$ ($\theta \sim 297°$) [8].

## SI-11. MONTE CARLO TEMPERATURE-DEPENDENCE SPIN STRUCTURE FACTORS

To supplement the temperature dependence of the spin structure factor reported in the main text in Fig. 2, we now provide the evolution of the spin structure factor as a function of temperature sampled via classical Monte Carlo simulations in Fig. SI-11.1. A comparison between this figure and Fig. 2 in the main text, which shows the SCGA results for the DQQ model, demonstrates how SCGA is able to capture physics of the DQQ model above $T^*$. More specifically, at high temperatures, an almost featureless structure factor is observed. As the temperature is lowered

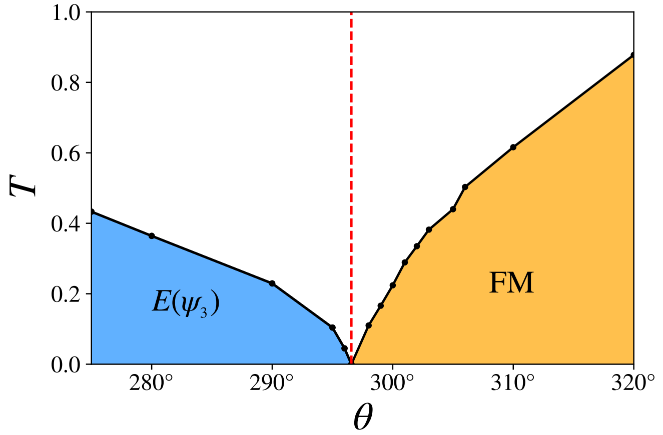


FIG. SI-10.1: Temperature-dependent phase diagram for the Heisenberg and DM model. Here, the red dashed line marks the DQQ model where no magnetic order is found down to the lowest temperatures considered.

in the range $T \in [T^*, T_{\rm gl}]$, the anisotropic twofold and fourfold pinch point features become more prominent and pinched. Finally, for temperatures below $T^*$, the fourfold pinch points disappear and a spin-ice pattern is obtained.

## SI-12. NEUTRON STRUCTURE FACTOR OF THE DQQ MODEL

In this section, we provide the polarized neutron structure factors in the $[hh\ell]$ and $[hk0]$ planes for the DQQ model obtained from our Monte Carlo simulations above and below the crossover temperature $T^*$ and obtained for the same temperatures as those used in Fig. 1 in the main text, see Fig. SI-12.1. Here, in calculating the neutron structure factor, and in wanting to make contact with potential experiments on non-Kramers ions, we have set the components of the $g$-tensor $g^{zz} = 1$ and $g^{\perp} = 0$ (see Section SI-3). We note that the polarized neutron structure factor in the spin-flip channel is similar to what would be observed for a spin-ice phase obtained from a nearest-neighbour Hamiltonian. In contrast, when studying the non-spin-flip channel a modulating pattern in the $[hh\ell]$ plane is observed for all the temperatures considered. This modulation is not typical of a simple nearest-neighbour Ising spin ice Hamiltonian where a featureless NSF in the $[hh\ell]$ plane is observed [4]. For Ising degrees of freedom, this modulation in the correlation functions can be obtained by considering an Ising antiferromagnetic model with further nearest-neighbour interactions [4]. The observation of this modulation in the DQQ model could be potentially associated with an effective Ising Hamiltonian where further nearest-neighbour terms are generated at low temperatures. We leave the study of the origin of this modulation for future work.

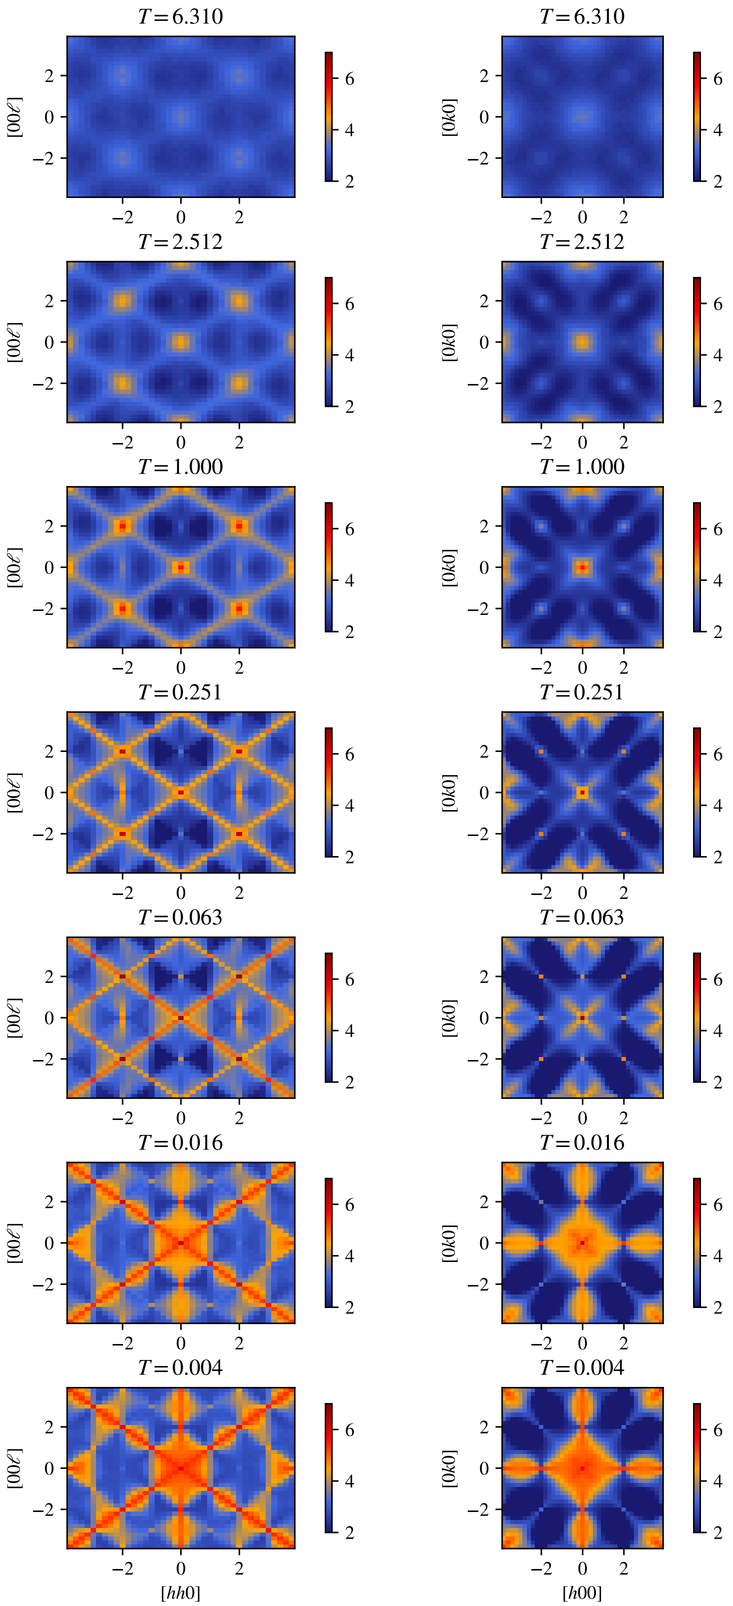


FIG. SI-11.1: Spin structure factor for the DQQ model in the $[hh\ell]$ (left column) and $[hk0]$ (right column) planes obtained via classical Monte Carlo, where each row corresponds to a different temperature shown above each panel. In this figure, only the last two rows correspond to correlation functions measured *below* the crossover temperature $T^*$.

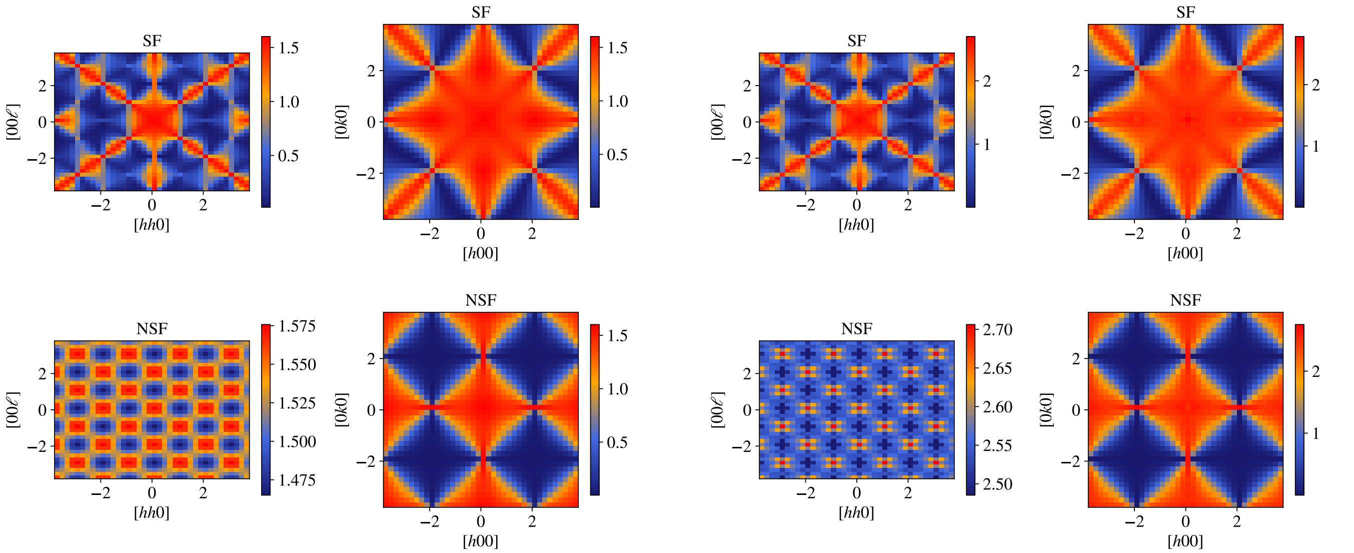


(a) $T > T^*$

(b) $T < T^*$

FIG. SI-12.1: Polarized neutron structure factors for the DQQ model above $T^*$ (a) at $T = 0.063J$ and below (b) at $T = 0.003J$ obtained from Monte Carlo. For both panels (a) and (b), the left plots correspond to the $[hh\ell]$ plane and the right plots to the $[hk0]$ plane where the first row is the spin-flip (SF) channel and the second row corresponds to the non-spin-flip (NSF) channel. These structure factors were obtained for a system size $L = 10$.

The PFFRG static neutron structure factor of the $S = 1/2$ model with interactions $\{J_{zz}, J_{\pm}, J_{\pm\pm}\} = \{3.0, 0.3, -1.0\}$ in the vicinity of the DQQ model is shown in Fig. SI-12.2. We note that the pattern in the non-spin flip channel differs from that of the classical DQQ model in the $[hh\ell]$ plane. Further information on the PFFRG method is provided below in Section SI-14.

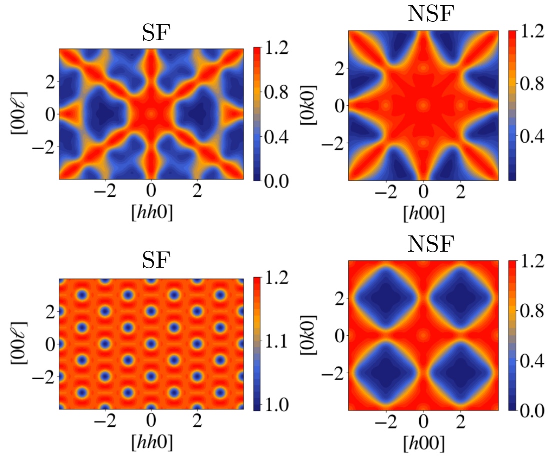


FIG. SI-12.2: PFFRG static polarized neutron structure factors for the model $\{J_{zz}, J_{\pm}, J_{\pm\pm}\} = \{3.0, 0.3, -1.0\}$. The first and second rows correspond to the spin-flip and non-spin-flip channels respectively.

## SI-13. DUAL DQQ MODEL (DQQ$^*$) SPIN STRUCTURE FACTORS

In the non-Kramers phase diagram shown in the inset of Fig. 1(a) in the main text, the DQQ model falls at a point where three phases meet: $T_1^{xy}$, $E$, and $T_1^{\rm Ice}$. As discussed in the main text, another triple point in the phase

diagram presented in Fig. 1(a) corresponds to the DQQ* model. The duality between these two points is generated by the transformation of the pseudo-spin operators $\hat{S}_i^{\pm} \to \pm i \hat{S}_i^{\pm}$, along with the change $J_{\pm\pm} \to -J_{\pm\pm}$, which leaves the non-Kramers Hamiltonian invariant. In terms of the spin components, this transformation amounts to a local rotation in the local $xy$ degrees of freedom [9]. This rotation has the effect of swapping the $T_1^{xy}$ irrep with the $T_2$ irrep as well as swapping the $\psi_2$ and $\psi_3$ components of the $E$ irrep, i.e. $T_1^{xy} \leftrightarrow T_2$ and $\psi_2 \leftrightarrow \psi_3$ (this symmetry is observed in the phase diagram in Fig. 1(a) where changing the sign of $J_{\pm\pm}$ has the effect of swapping the $T_2$ with the $T_1^{xy}$ phase). As a consequence of this duality, the DQQ* model has identical thermodynamic behaviour to the DQQ model, and an equivalent long-wavelength theory as the one presented in the main text.

Indeed, at temperatures below $T^*$, the dual model also exhibits a spin-ice phase with a spin structure factor resembling the ones obtained for the DQQ model in Fig. 1(e) and (f). In contrast, and as a consequence of the local pseudo-spin transformation, the spin structure factor of the DQQ* model *above* $T^*$ does not match the one obtained for the DQQ model, see Fig. SI-13.1. The similarity at low temperatures and disagreement at high temperatures can be understood by the local transformation $\hat{S}_i^{\pm} \to \pm i \hat{S}_i^{\pm}$: since this duality transformation only involves the local $xy$ spin degrees of freedom, the structure factor below $T^*$, mostly generated by spin-ice configurations with *only* local $z$ components, is the same, whereas the structure factor above $T^*$ differs as the thermal $xy$ fluctuations contributing in the DQQ and DQQ* models are different.

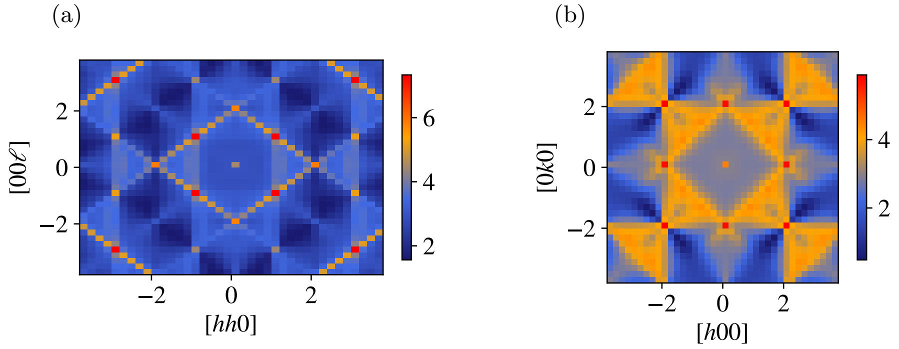


FIG. SI-13.1: Spin structure factors for the dual model (DQQ*) just above the temperature $T^*$. Panel (a) corresponds to the $[hh\ell]$ plane and panel (b) to the $[hk0]$ plane. These structure factors were obtained for a system size $L = 10$.

## SI-14. PSEUDO-FERMION FUNCTIONAL RENORMALIZATION GROUP (PFFRG) METHOD

The PFFRG [14–16] is a variant of functional renormalization group (FRG) approaches [17] which introduces a cutoff (e.g. frequency cutoff) $\Lambda$ to the fermionic free propagator of a model in order to derive a set of coupled differential equations for cutoff dependent $n$-particle vertex functions. Each so-called flow equation for the $n$-particle vertex couples the latter to the $(n+1)$ particle vertex. While the untruncated flow equations are exact, a numerical solution requires a truncation above the $n$-particle level. After applying a truncation of the flow equations, in our case the so-called one-loop plus Katanin truncation [16], the flow equations are solved from the known infrared cutoff limit towards the cutoff-free model. In order to apply the FRG framework to spin models, within PFFRG, spins are mapped onto pseudo-fermions via

$$S_i^{\mu} = \frac{1}{2} \sum_{\alpha\beta} f_{i\alpha}^{\dagger} \sigma_{\alpha\beta}^{\mu} f_{i\beta}, \tag{S1}$$

where $f_{i\alpha}$, $f_{i\alpha}^{\dagger}$ are fermion operators on site $i$ with $\alpha, \beta = \uparrow, \downarrow$ and $\sigma^{\mu}$ are Pauli matrizes with $\mu = x, y, z$. The mapping introduces unphysical states in the form of non- and doubly- occupied sites. The method is applied at zero temperature to keep the influence of unphysical states on the ground state at a minimum.

The PFFRG flow equations provide the fermionic self-energy and two-particle vertex, which allow for the computation of the magnetic susceptibility. The various symmetries of the models considered are implemented on an exact level such that the susceptibility is expected to diverge at the critical cutoff of a magnetic phase transition. Instead, within a numerical solution, the susceptibility flow usually breaks down upon approaching a phase transition, visible as a kink in the susceptibility flow, before a divergence can manifest. Susceptibilities at cutoffs below the breakdown are unphysical. Vice versa, the absence of a susceptibility breakdown throughout the flow is interpreted as an absence of magnetic order at zero temperature. However, especially near phase boundaries, renormalization group flows may neither show a clear breakdown nor a smooth flow down to $\Lambda \to 0$, such that the identification as magnetic versus paramagnetic can become ambiguous. These regions are marked as white areas in the phase diagram of the quantum model Fig 5(a) in the main text.

The PFFRG is currently only formulated for models with time-reversal symmetry [16], such that finite magnetic order parameters cannot be probed. Instead, the irrep formalism, applied to the present nearest-neighbour spin model on the pyrochlore lattice, is used to specify magnetic orders by identifying the maximum order parameter susceptibility, given by E(9) in the main text, just above the critical cutoff [8]. In absence of magnetic order at $T = 0$, high order parameter susceptibilities signify which irrep manifolds are most relevant to the paramagnetic ground state.

## SI-15. PFFRG SPIN STRUCTURE FACTORS IN THE VICINITY OF THE DQQ POINT

We show the PFFRG static spin structure factors of models in the paramagnetic and uncertain region of the quantum model phase diagram Fig. 5(a) (in main text) near the DQQ model in Fig. SI-15.1. The plots are obtained in the low-cutoff limit of $\Lambda = 0.02J_{zz}$.

## SI-16. HIGH-TEMPERATURE SERIES EXPANSION (HTSE)

To calculate the susceptibilities for some magnetic order labeled $\psi$, we consider the spin-half model in the thermodynamic limit and add to the Hamiltonian an infinitesimal (conjugate) field term that couples to the order parameter of interest, $M_\psi$,

$$\mathcal{H}_\psi = -h_\psi M_\psi. \tag{S1}$$

The susceptibility per site is defined in terms of the partition function $Z(h_\psi)$ as

$$\chi = -\frac{1}{N}\frac{1}{T}\frac{\partial^2}{\partial h_\psi^2}\ln Z(h_\psi)\big|_{h_\psi=0}. \tag{S2}$$

We have calculated the high-temperature series expansion for the $T_1^{xy}$ and $E$ susceptibilities to order $\beta^8$ ($\beta \equiv 1/T$) along several different paths varying $J_{\pm\pm}$ and for various values of $J_\pm$ while keeping $J_{zz} = 3$.

The leading order of the expansion, when expressed as a series for the inverse susceptibility gives

$$\frac{1}{\chi} = \frac{4}{\beta}(1 - \theta_\psi \beta), \tag{S3}$$

which can be re-expressed as the Curie-Weiss law:

$$\chi = \frac{0.25}{T - \theta_\psi}. \tag{S4}$$

We find that the Curie-Weiss temperature is larger for the $T_1^{xy}$ and $E$ susceptibilities inside their respective classical phases. The two Curie-Weiss constants become equal along the classical phase boundary $J_{\pm\pm} = -2J_\pm$. This shows the equivalence of the quantum and classical models at the Curie-Weiss (mean-field) level.

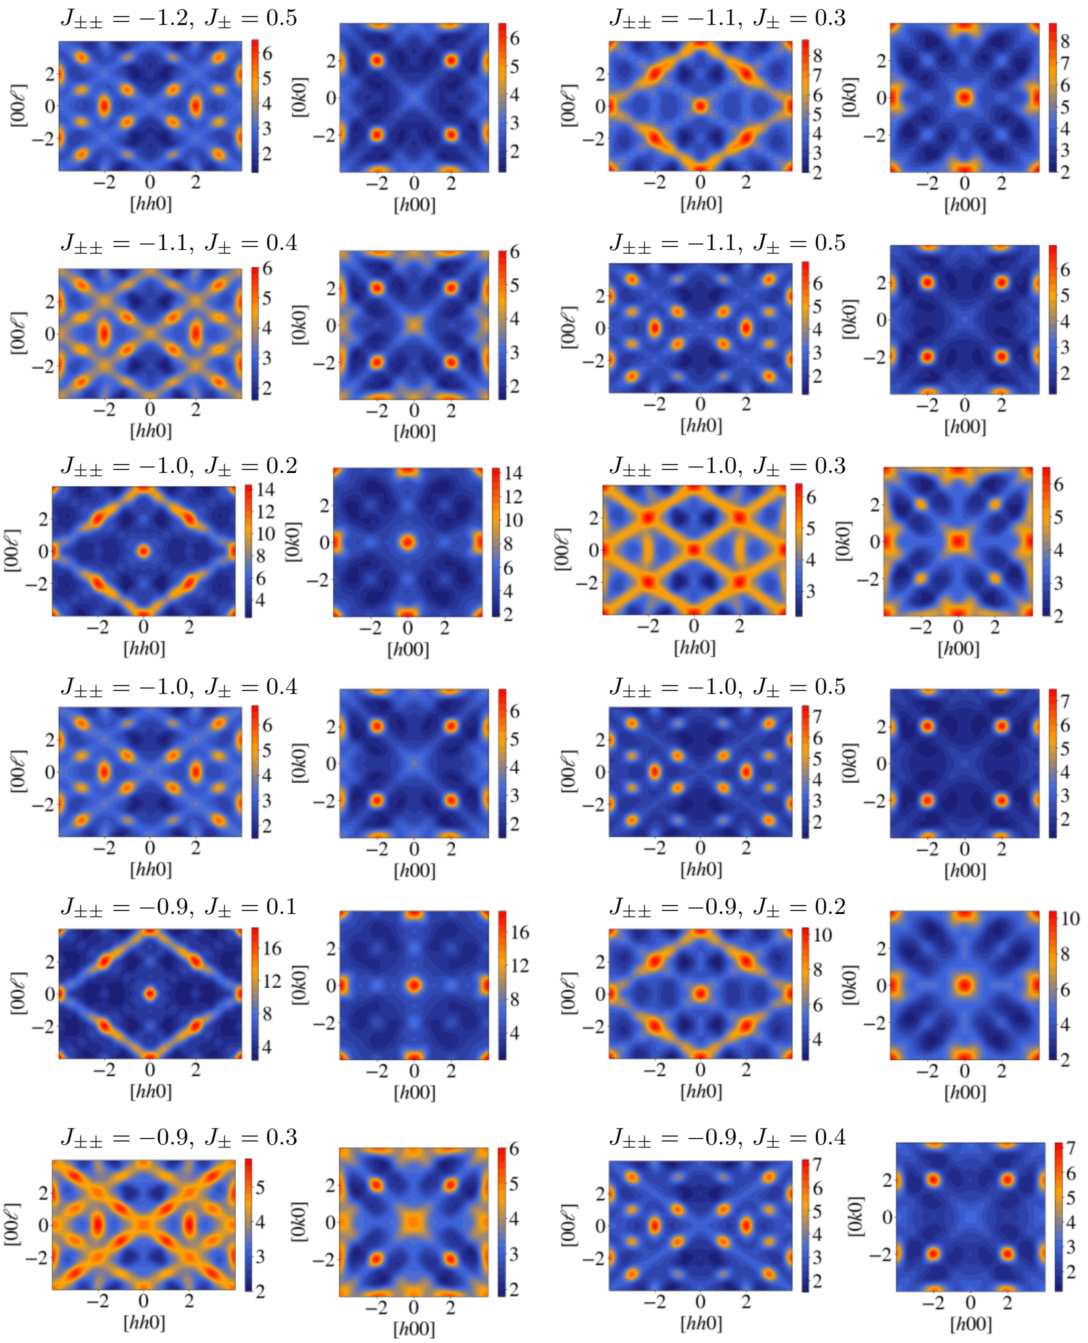


FIG. SI-15.1: PFFRG static spin structure factors in the low cutoff limit. Different interactions with constant $J_{zz} \equiv 3$, and within the paramagnetic regime of the quantum model phase diagram Fig. 5 in the main text near the DQQ model are considered.

To analyze the series to order $\beta^8$, we construct Padé approximants [18], with a number of approximants being calculated. We select three to five approximants for each $\{J_\pm, J_{\pm\pm}\}$ parameters that show best convergence down to temperatures of order unity (in units of $J$). The susceptibilities are shown in Fig. SI-16.1. Along each $J_{\pm\pm}$ line, we pick one parameter value that falls in the classical $E$ phase, one on the classical phase boundary and several parameter values in the classical $T_1^{xy}$ phase. Susceptibilities are shown for four different $J_\pm$ values for each $J_{\pm\pm}$ value. For a given $J_{\pm\pm}$ the color corresponds to the $J_\pm$ values. Three of the $J_\pm$ values are common between the $T_1^{xy}$ and $E$ susceptibility plots so they can be directly compared. We find that even along the classical phase boundary the

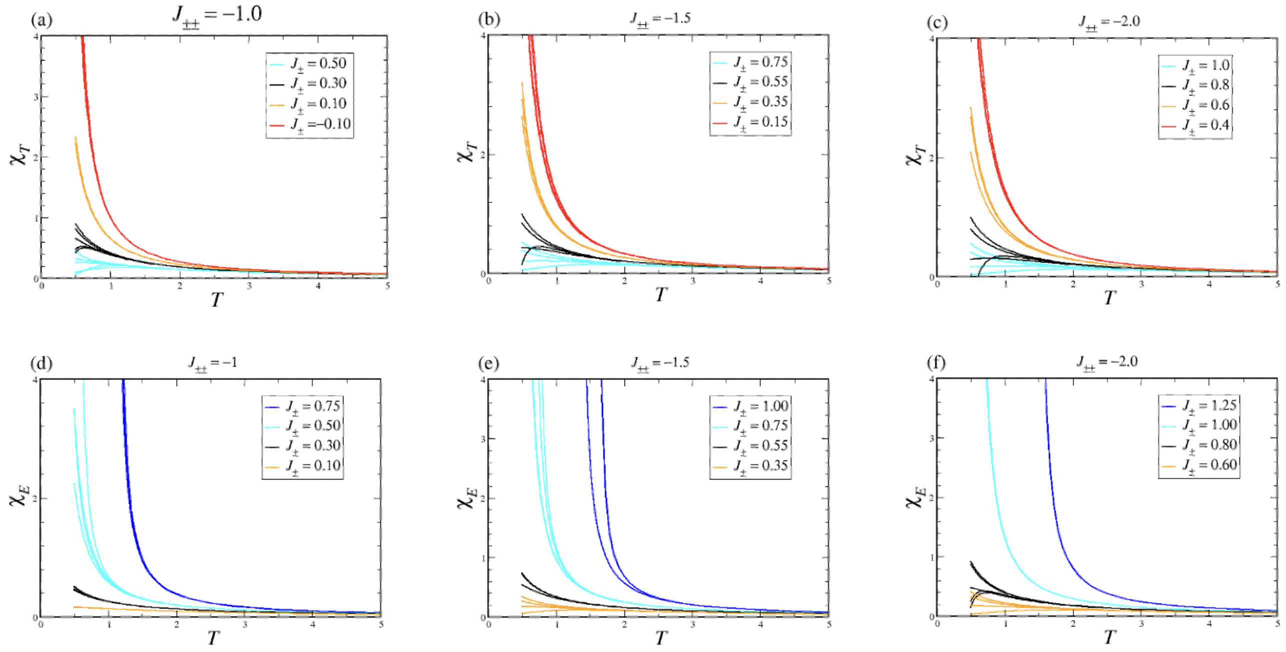


FIG. SI-16.1: Figures (a)-(c) show susceptibility $\chi_T$ for the $T_1^{xy}$ order and figures (d)-(f) show susceptibility $\chi_E$ for the $E$ order. Three to five different Padé approximants are shown for each parameter. Different colors correspond to different sets of exchange parameters. The blue color corresponds to a point inside the classical $E$ phase, the cyan color to a point along the classical phase boundary, the black color is inside the classical $T_1^{xy}$ phase and the orange and red colors are deeper in the $T_1^{xy}$ phase. Both sets of susceptibilities are shown for a same set of parameters for cyan, black and orange cases. For example, for $J_{\pm\pm} = -1.0$, $\chi_E$ and $\chi_T$ are both computed, and shown, for $J_{\pm} = 0.5, 0.3,$ and 0.10. The susceptibility $\chi_E$ becomes large inside the classical $E$ phase (blue), along the classical phase boundary (cyan) and a little into the classical $T_1^{xy}$ phase. On the other hand, one needs to go someways into the classical $T_1^{xy}$ phase to see the growth in $\chi_T$ (orange and red colors). In between there is a corridor in parameter space running parallel to the classical phase boundary where neither susceptibility shows growth (black curves). See Fig. 5(a) in the main text.

tendency towards $E$ order grows rapidly as temperature is lowered. The $T_1^{xy}$ susceptibility only grows rapidly once we are some ways into the classical $T_1^{xy}$ phase and away from the classical phase boundary; see Fig. 5(a) in the main text. This behavior is in very good agreement with the PFFRG calculations. In between, a corridor opens up separating the $E$ and $T_1^{xy}$ phases that runs parallel to the classical phase boundary, where neither susceptibility grows rapidly upon cooling.

---


[1] T. Moriya, Anisotropic Superexchange Interaction and Weak Ferromagnetism, Physical Review **120**, 91 (1960).

[2] T. Moriya, New mechanism of anisotropic superexchange interaction, Phys. Rev. Lett. **4**, 228 (1960).

[3] I. Dzyaloshinsky, A thermodynamic theory of "weak" ferromagnetism of antiferromagnetics, Journal of Physics and Chemistry of Solids **4**, 241 (1958).

[4] K. T. K. Chung, J. S. K. Goh, A. Mukherjee, W. Jin, D. Lozano-Gómez, and M. J. P. Gingras, Probing flat band physics in spin ice systems via polarized neutron scattering, Phys. Rev. Lett. **128**, 107201 (2022).

[5] S. Lee, S. Onoda, and L. Balents, Generic quantum spin ice, Phys. Rev. B **86**, 104412 (2012).

[6] H. Kadowaki, H. Takatsu, T. Taniguchi, B. Fåk, and J. Ollivier, Composite spin and quadrupole wave in the ordered phase of $Tb_{2+x}Ti_{2-x}O_{7+y}$, SPIN **05**, 1540003 (2015).

[7] H. Yan, O. Benton, L. Jaubert, and N. Shannon, Theory of multiple-phase competition in pyrochlore magnets with anisotropic exchange with application to $Yb_2Ti_2O_7, Er_2Ti_2O_7$, and $Er_2Sn_2O_7$, Phys. Rev. B **95**, 094422 (2017).

[8] V. Noculak, D. Lozano-Gómez, J. Oitmaa, R. R. P. Singh, Y. Iqbal, M. J. P. Gingras, and J. Reuther, Classical and quantum phases of the pyrochlore $S = \frac{1}{2}$ magnet with Heisenberg and Dzyaloshinskii-Moriya interactions, Phys. Rev. B **107**, 214414 (2023).

[9] J. G. Rau and M. J. P. Gingras, Frustrated quantum rare-earth pyrochlores, Annu. Rev. Condens. Matter Phys. **10**, 357 (2019).

[10] S. V. Isakov, K. Gregor, R. Moessner, and S. L. Sondhi, Dipolar Spin Correlations in Classical Pyrochlore Magnets, Phys. Rev. Lett. **93**, 167204 (2004).

[11] P. H. Conlon and J. T. Chalker, Absent pinch points and emergent clusters: Further neighbor interactions in the pyrochlore Heisenberg antiferromagnet, Phys. Rev. B **81**, 224413 (2010).

[12] D. Lozano-Gómez, *Symmetry breaking, order by disorder, fragmentation, and spin liquids in the magnetic pyrochlore lattice with anisotropic interactions*, Ph.D. thesis, University of Waterloo (2023), Ph.D. thesis, University of Waterloo, (2023).

[13] L. R. Walker and R. E. Walstedt, Computer model of metallic spin-glasses, Phys. Rev. B **22**, 3816 (1980).

[14] J. Reuther and P. Wölfle, $J_1 - J_2$ frustrated two-dimensional Heisenberg model: Random phase approximation and functional renormalization group, Phys. Rev. B **81**, 144410 (2010).

[15] F. L. Buessen, V. Noculak, S. Trebst, and J. Reuther, Functional renormalization group for frustrated magnets with nondiagonal spin interactions, Phys. Rev. B **100**, 125164 (2019).

[16] T. Müller, D. Kiese, N. Niggemann, B. Sbierski, J. Reuther, S. Trebst, R. Thomale, and Y. Iqbal, Pseudo-fermion functional renormalization group for spin models (2023), arXiv:2307.10359 [cond-mat.str-el].

[17] W. Metzner, M. Salmhofer, C. Honerkamp, V. Meden, and K. Schönhammer, Functional renormalization group approach to correlated fermion systems, Rev. Mod. Phys. **84**, 299 (2012).

[18] J. Oitmaa, C. Hamer, and W. Zheng, *Series Expansion Methods for Strongly Interacting Lattice Models* (Cambridge University Press, 2006).
